# Supplementary material for: A tale of two phase diagrams: Interplay of ordering and hydrogen uptake in Pd-Au-H
Source: arXiv:2103.14340 ancillary file (2021-03-26)
Supplement: Supplementary file 1 [file supplementary-information.pdf]

# A tale of two phase diagrams: Interplay of ordering and hydrogen uptake in Pd–Au–H

J. Magnus Rahm, Joakim Löfgren, Erik Fransson, and Paul Erhart

## Contents

|                                                                                                 |           |
|-------------------------------------------------------------------------------------------------|-----------|
| <b>Notes</b>                                                                                    | <b>2</b>  |
| SN1. Construction of phase diagram in full equilibrium . . . . .                                | 2         |
| <b>Figures</b>                                                                                  | <b>3</b>  |
| S1. Plateau pressures in pure Pd . . . . .                                                      | 3         |
| S2. Relaxations and shearing in PdAu:H . . . . .                                                | 3         |
| S3. RMSE, AIC, and BIC as a function of cutoffs in the cluster expansion . . . . .              | 4         |
| S4. Prior and posterior distributions for hyper parameters . . . . .                            | 5         |
| S5. Corner plot for the most short-ranged ECIs . . . . .                                        | 6         |
| S6. Critical temperatures of L <sub>12</sub> with and without hydrogen . . . . .                | 7         |
| S7. Change in uptake of hydrogen and SRO with annealing temperature . . . . .                   | 7         |
| S8. SRO in full equilibrium . . . . .                                                           | 8         |
| S9. LRO in full equilibrium . . . . .                                                           | 8         |
| S10. Phase diagram in full equilibrium at 250 K and 500 K . . . . .                             | 9         |
| S11. Change in hydrogen uptake with annealing temperature and H <sub>2</sub> pressure . . . . . | 9         |
| <b>References</b>                                                                               | <b>10</b> |

## Notes

### Supplementary Note 1: Construction of phase diagram in full equilibrium

To construct the phase diagram in full equilibrium, we made Monte Carlo (MC) simulations in which we sampled the variance-constrained semi-grand canonical (VCSGC) ensemble on both lattices. We thus had two independent parameters  $\bar{\phi}$ , one per sublattice, with which we could sweep (in steps of  $\Delta\bar{\phi} = 0.04$ ) the full 2D concentration range. This yielded two partial free energy derivatives,

$$\frac{\partial F}{\partial c_{\text{Au}}} \quad \text{and} \quad \frac{\partial F}{\partial c_{\text{H}}}. \quad (1)$$

To compute the free energy, we may integrate Equation 1 along some 2D path. Ideally, the choice of integration path is unimportant; they should all yield the same result. Nevertheless, noise in the MC results can quickly accumulate, resulting in different results depending on integration path. Furthermore, a long integration path runs a higher risk of accumulating a lot of noise. To overcome these challenges, we defined a 2D grid of points between 0 and 70% H, and 0 and 50% Au, both in steps of 5%. We then linearly interpolated the free energy derivatives (Equation 1) on a denser grid (spacing 1%). Starting from a point on the sparse grid, we then defined 10 different integration paths to each point on the dense grid. These paths were constructed by taking the required number of steps needed in the  $c_{\text{Au}}$  and the  $c_{\text{H}}$  direction in a random order (following a “taxicab geometry”). We averaged the results over these 10 paths, and constructed the convex hull and recorded all points on the dense grid that were on the convex hull. This process was repeated for all starting points on the sparse grid. In the end, each point on the dense grid had been recorded as belonging to the convex hull a certain number of times, between 0 and the number of starting points on the sparse grid. To finally plot the phase diagram, we removed all the points that had been recorded on the convex hull less than 5% of the point that been recorded the most number of times, and finally plotted the result as a heat map with colors logarithmically dependent on how many times each point was recorded on the convex hull.

Finally isobars were drawn by identifying the points at which the interpolated derivatives  $\partial F/\partial c_{\text{H}} = \mu_{\text{H}}$  attained the value corresponding to the sought pressure. Whenever these points crossed a multi-phase region, they were replaced with a straight line starting/ending where the isobar left/entered a single-phase region.

## Figures

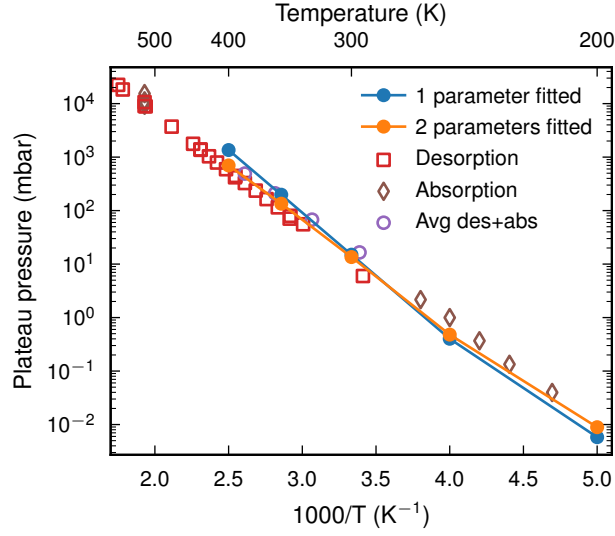

**Figure S1:** Plateau pressure in absorption and desorption isotherms of hydrogen in pure Pd. Red squares, brown diamonds and purple circles are, respectively, experimental desorption, absorption and average desorption/absorption pressures from the literature (1–5). Orange line is our two-parameter fit as described in the main paper. Blue line is a one-parameter fit, where the first-degree polynomial described in the main paper is replaced by a constant.

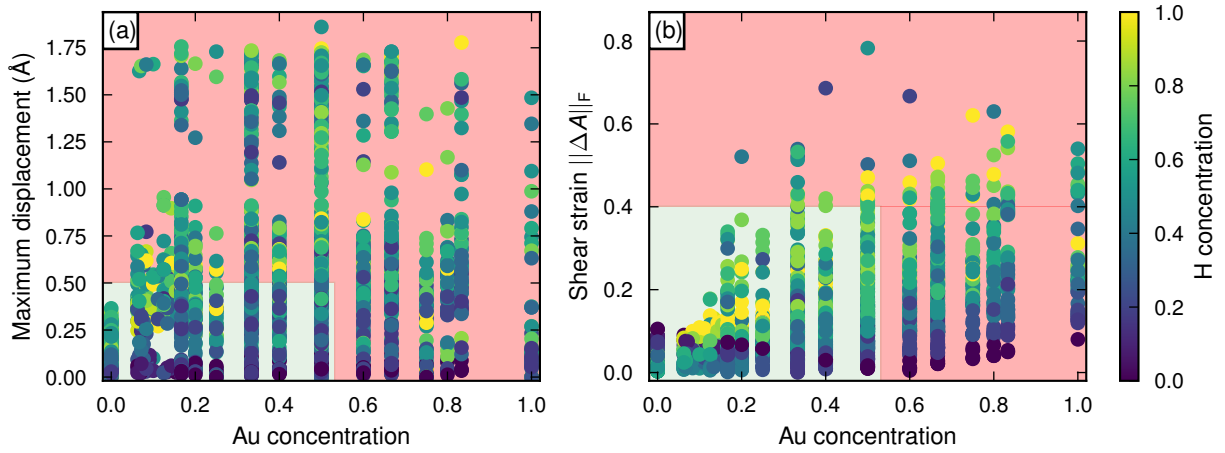

**Figure S2:** Relaxations from ideal rocksalt structure in PdAu:H. Relaxation is split in (a) maximum displacement from ideal lattice site among the atoms in the structure and (b) shearing of the cell as measured by the Frobenius norm of the shear part of the transformation  $\|\Delta A\|_F$ . Each dot represents one atomic structure, and its color represents the H content. Atomic structures in the light red areas were not used for training of the cluster expansion (CE).

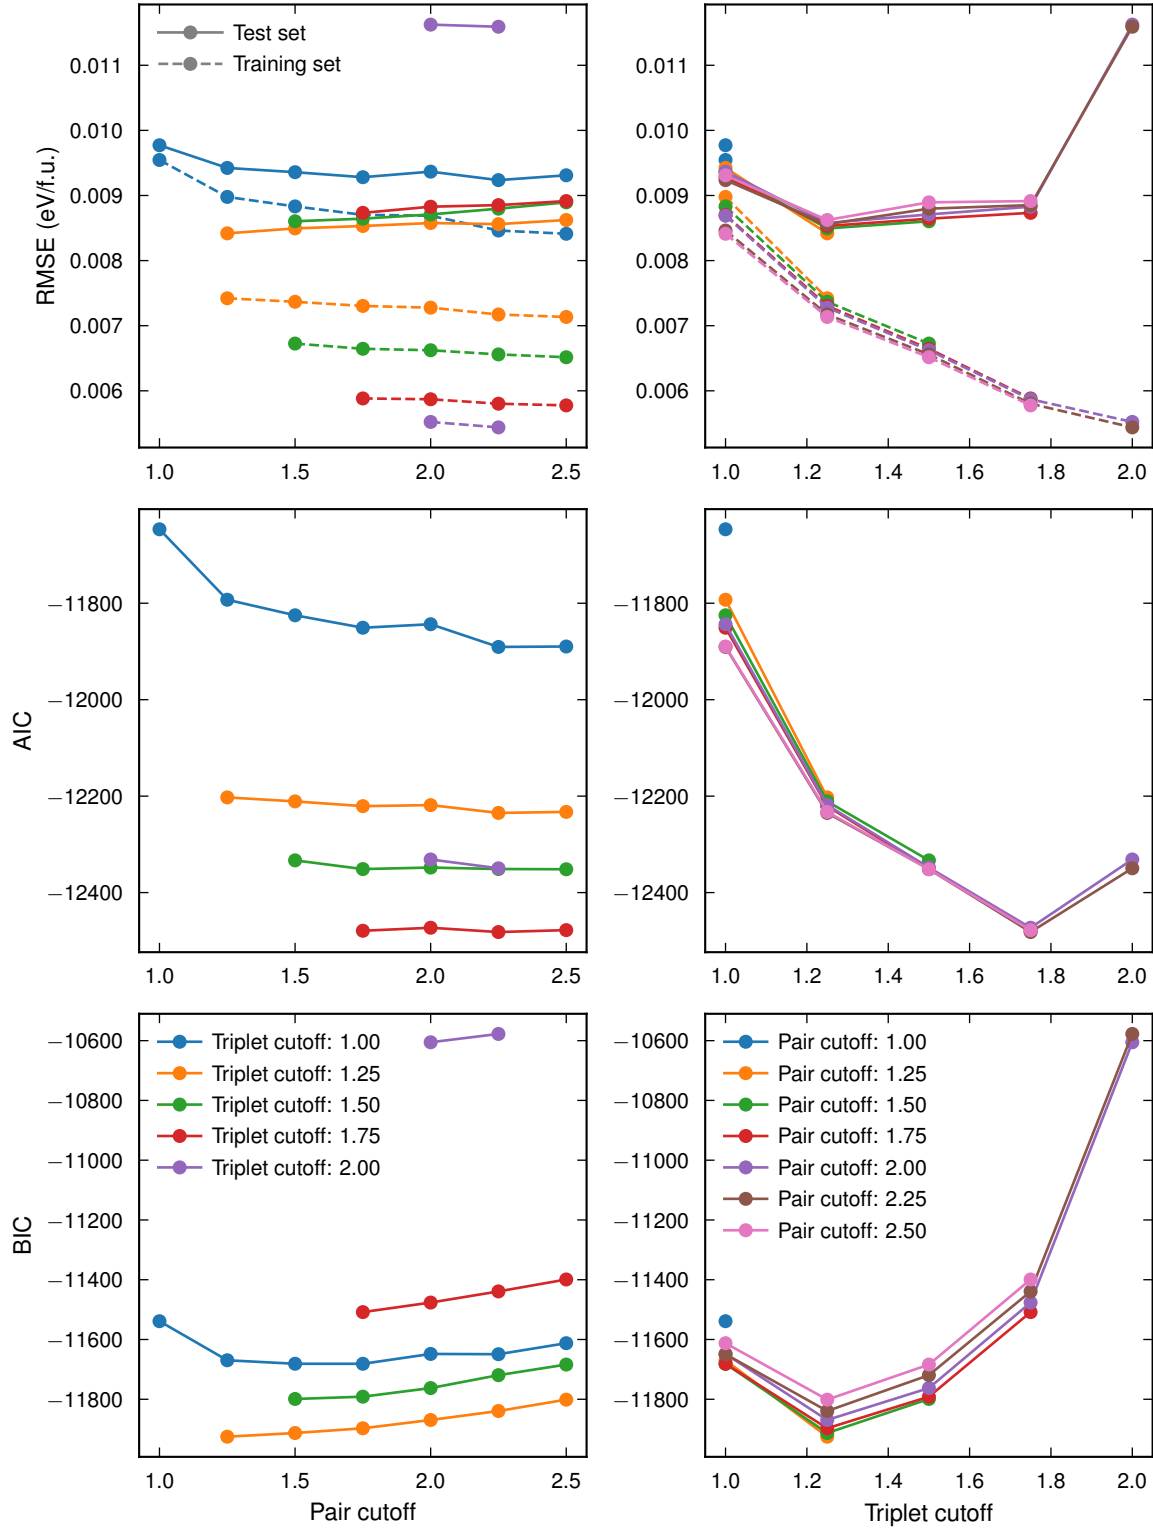

**Figure S3:** Root mean square error (RMSE, top row), Akaike information criterion (AIC, middle row), and Bayesian information criterion (BIC, bottom row) as a function of pair (left column) and triplet cutoff (right column) in the truncation of the CE. Cutoffs are given in units of the lattice parameter, and specify the longest allowed interatomic distance in the cluster. The different criteria paint slightly different pictures, but a pair cutoff at 1.75 was deemed reasonable as it provides a low RMSE in the test set and one of the lowest AIC and BIC values, and a triplet cutoff at 1.25 was chosen as it minimizes the RMSE of the training set and the BIC. To produce this data, the non-weighted training set was fitted with ordinary least squares, and the RMSE values are therefore slightly lower than for the final CE.

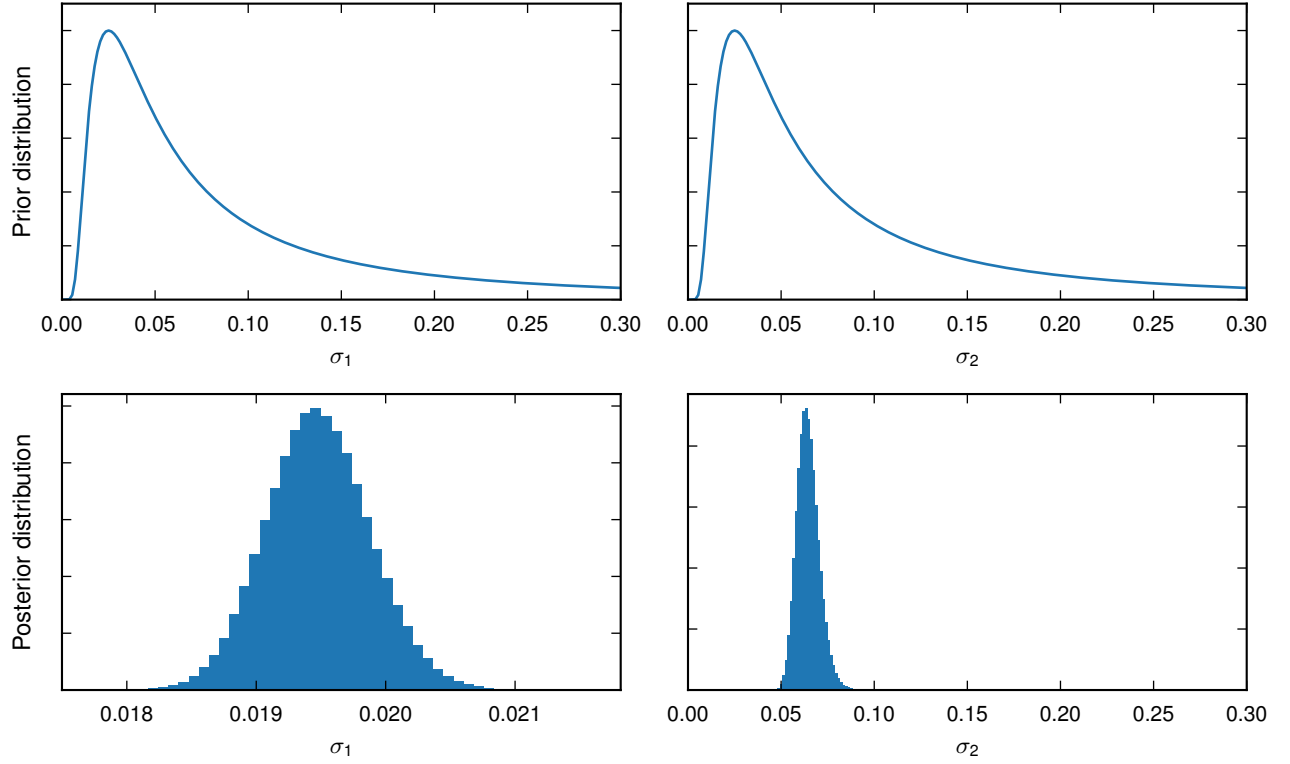

**Figure S4:** Prior distributions (top row) and posterior distributions (bottom row) for the hyper parameters  $\sigma_1$  (left column) and  $\sigma_2$  (right column). The parameter  $\sigma_1$  is defined by assuming that the errors, defined as the difference between the DFT energy and the CE energy, are normally distributed with zero mean and variance  $\sigma_1^2$ . The posterior distribution for  $\sigma_1$  thus indicates the magnitude of the error in the model, but note that  $\sigma_1$  relates to errors after weighting according to Au concentration and the real error is therefore smaller than what  $\sigma_1$  indicates. The parameter  $\sigma_2$  is defined as the variance of the normally distributed prior for the ECIs.

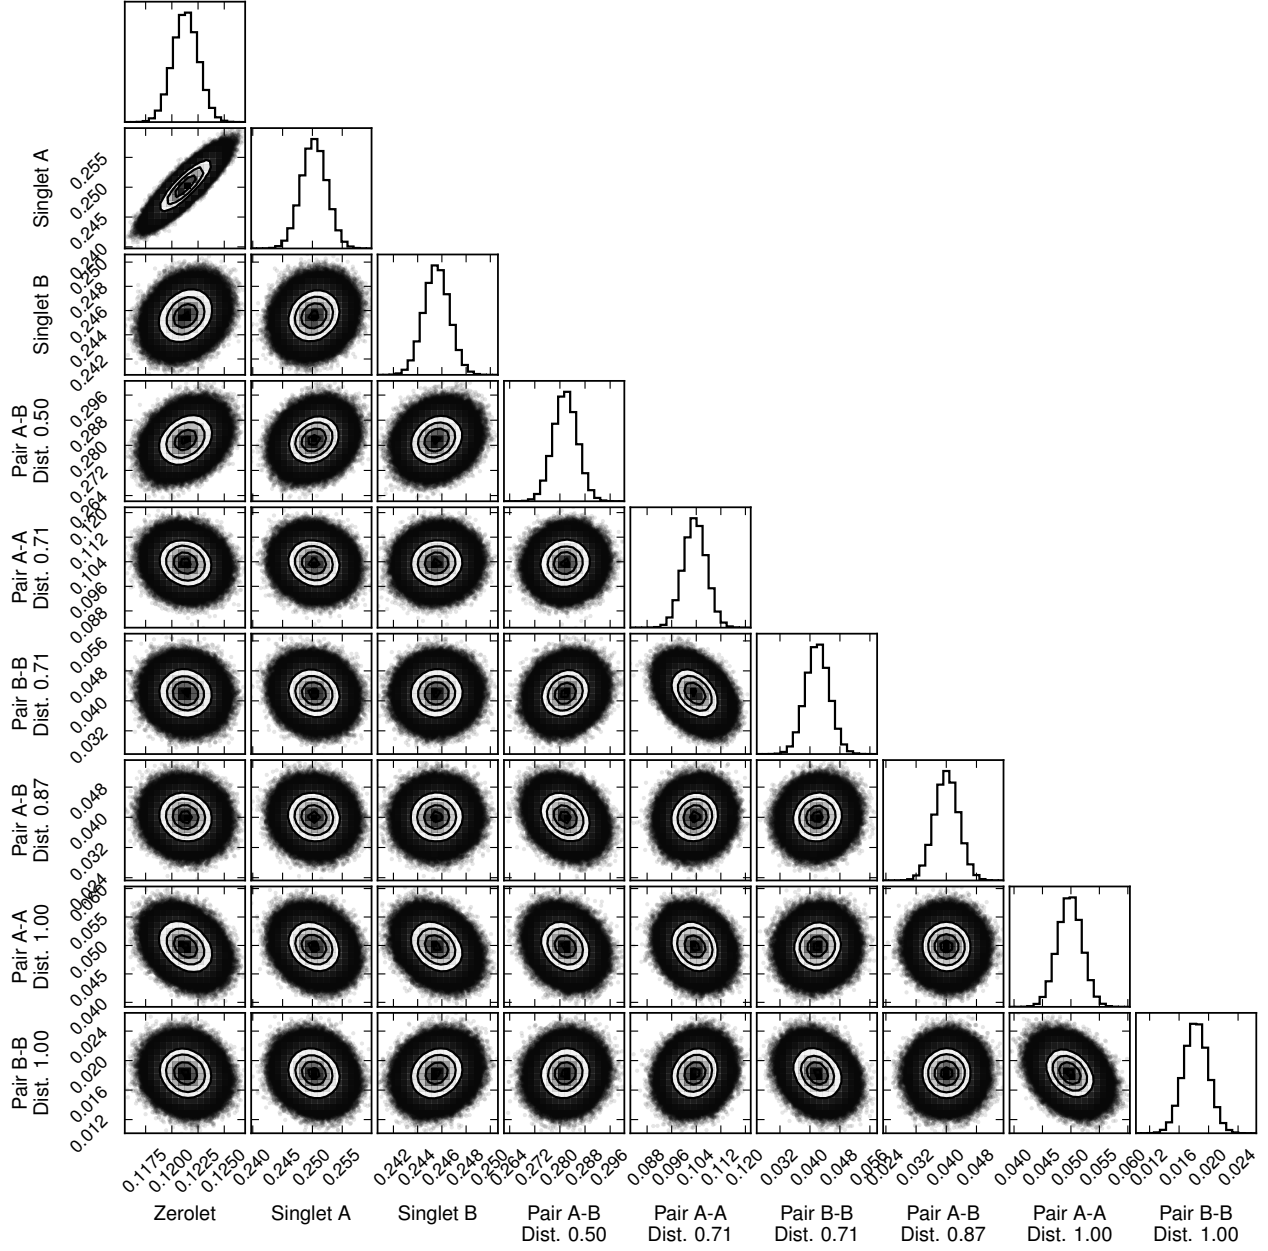

**Figure S5:** Corner plot (6) for the 9 most short-ranged ECIs (in units of eV/formula unit), showing the posterior distribution for each ECI (plots on the diagonal) as well as the correlation between each pair of ECIs. A and B in the labels refer, respectively, to the Pd–Au and H–vacancy sublattices. For example, A–A means that the ECI describes an energy related to the interaction between Au/Pd and Au/Pd. The labels also specify the distance between the atoms in each pair in units of the lattice parameter.

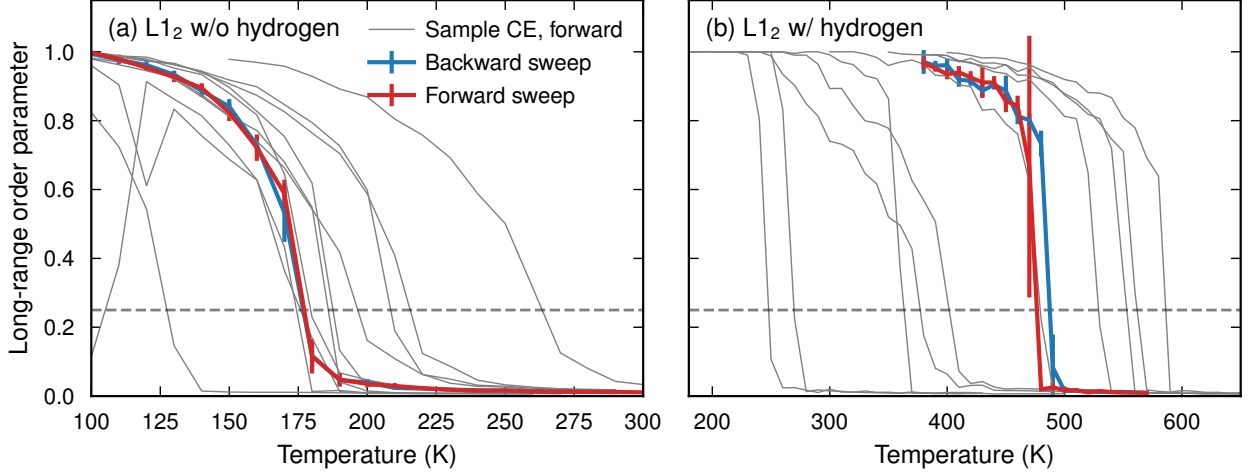

**Figure S6:** Estimation of critical temperature for the  $L1_2$  phase without hydrogen (a) and with 25% hydrogen (b). For these calculations, MC simulations were run in the canonical ensemble on the Pd–Au sublattice in (a) and on both sublattices in (b). The simulations were commenced from either the perfectly ordered phase and low temperature or a solid solution and high temperature, and the temperature was then, respectively, increased (“forward”) or decreased (“backward”), in steps of 10 K using 500 MC sweeps at each temperature. This was done with the CE developed in this work (red and blue lines) as well as with ten sampled CEs (grey lines, only forward sweep shown). Long-range order (LRO) was quantified by the structure factor  $S(\mathbf{q})$  (see main paper) using the maximum value of the three symmetrically equivalent versions of  $\mathbf{q} = 2\pi/a_0(1, 0, 0)$ , and normalized such that perfect order means order parameter equals 1. The critical temperature was estimated as the average of the temperatures where the forward and backward sweep reached 25% of maximum LRO. For a few of the sample CEs, the critical temperature in the hydrogen-free case was too low to be reliably sampled with this method, and the lines are discontinuous at low temperatures.

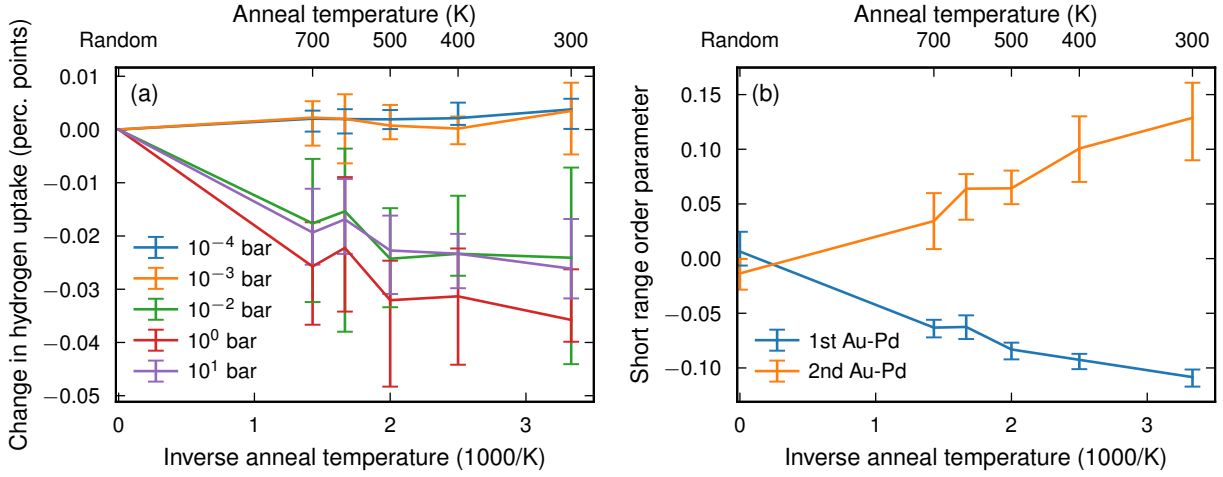

**Figure S7:** Change in uptake of hydrogen (a) at 300 K for Pd–Au with 25% Au as equilibrated at different temperatures (without hydrogen). The change in uptake depends on the loading pressure of  $H_2$ , as is the strongest at approximately 1 bar (red line). The difference between the Pd–Au structures after annealing in different temperatures can be quantified by the short-range order (SRO) parameter (b) for the first (blue line) and second (orange) nearest-neighbor Pd–Au pair. The data was generated by a hydrogen-free simulation in the canonical ensemble at the respective temperature, and five snapshots were randomly selected from those trajectories. These Pd–Au structure of these snapshots was then frozen, and subjected to a simulation in the semi-grand canonical (SGC) ensemble on the H–vacancy sublattice, using chemical potential corresponding to the pressures specified in the legend in (a). Error bars indicate the spread over the five different structures, lines their average.

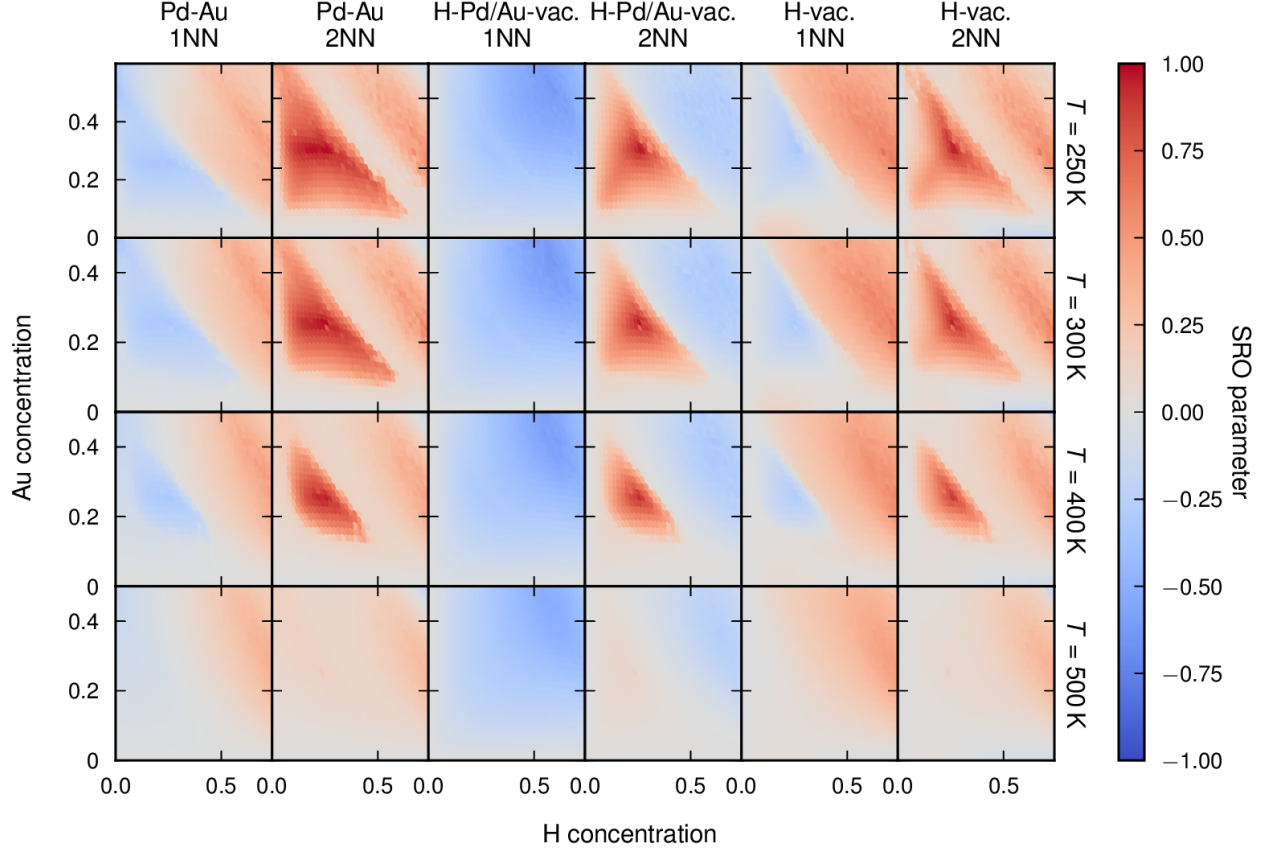

**Figure S8:** Short-range order (SRO) in full equilibrium as obtained with VCSGC-MC simulations at 250 K (top row), 300 K (second row), 400 K (third row), and 500 K (bottom row). Note that while this plot represents a single-phase region everywhere, the phase diagram predicts that in some regions, we expect phase separation. The ordered  $L1_2$  phase is typically not clearly exhibited in the first nearest neighbor (1NN) shell. While this may appear unexpected in particular for the 1NN H-Pd/Au-vac. pair SRO, given that the ordered phase has hydrogen surrounded by Pd only, this is an effect of the fact that vacancies are included in the SRO, and they have a mix of Pd and Au nearest neighbors. Instead, the perfectly ordered phase correspond to  $SRO = 1$  in the second shell in all three sublattices (vacancies have only Pd and Pd have only Au next nearest neighbors, for example). Further note that in several cases (1 NN Pd-Au, 2 NN H-vacancy, 1 NN H-vacancy), the SRO changes sign when the high-pressure (upper right half) region is entered.

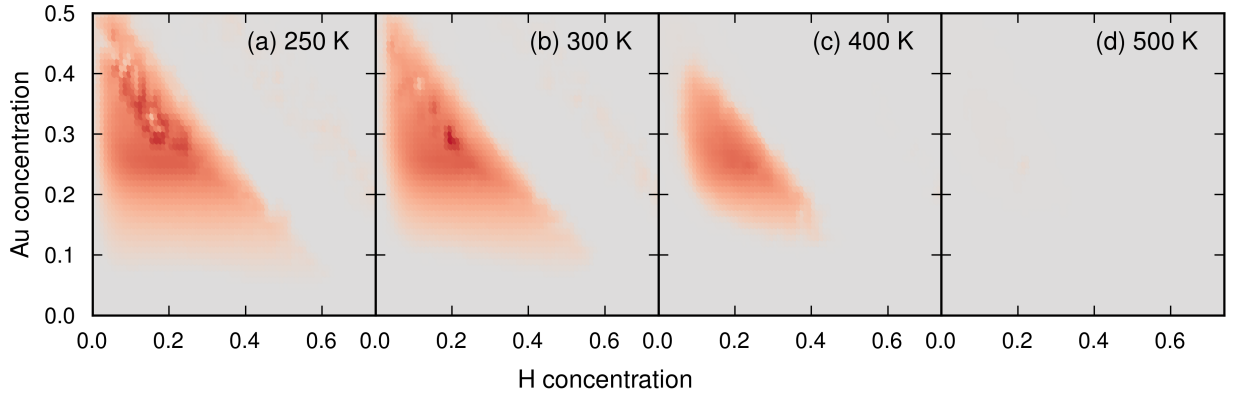

**Figure S9:** LRO parameter in full equilibrium at 250 K (a), 300 K (a), 400 K (a), and 500 K (d), quantified by the structure factor  $S(\mathbf{q})$  (see main paper) using the maximum value of the three symmetrically equivalent versions of  $\mathbf{q} = 2\pi/a_0(1, 0, 0)$ . Red color indicates more order, gray color is complete lack of order.



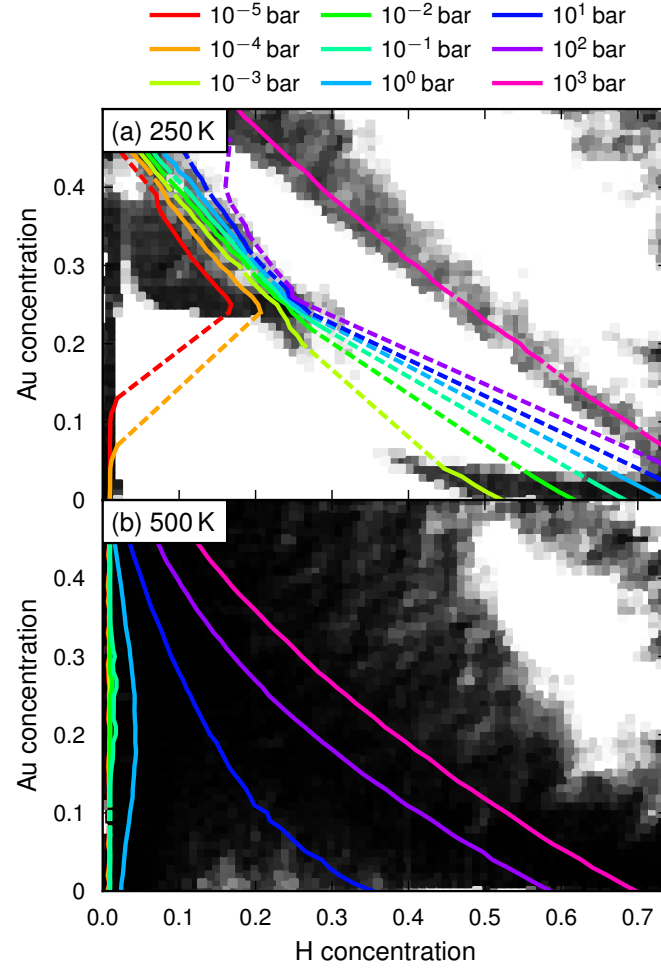

**Figure S10:** Phase diagram in equilibrium at 250 K (a) and 500 K (b).

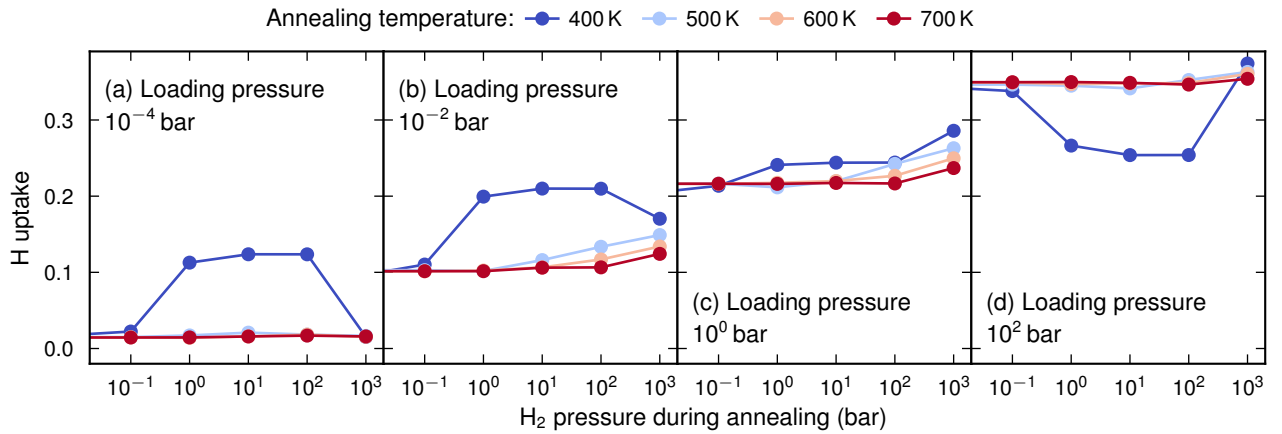

**Figure S11:** Hydrogen uptake at 300 K and H<sub>2</sub> pressure 10<sup>-4</sup> bar (a), 10<sup>-2</sup> bar (b), 1 bar (c), and 100 bar (d), in Pd–Au with 25% Au annealed at different temperatures (corresponding to different lines) and at different H<sub>2</sub> pressures (the abscissa). When annealing in 400 K (dark blue lines), the L1<sub>2</sub> phase forms at H<sub>2</sub> pressures between 1 and 100 bar, and this phase absorbs a significantly larger amount of hydrogen at 300 K and low pressures (a–b), whereas at high pressures it absorbs less than the solid solution Pd–Au (d). Very high H<sub>2</sub> pressures during annealing (at least 10 bar) are required to make a significant change to the hydrogen uptake if this ordered phase does not form.

## References

- [1] H. Frieske and E. Wicke, *Magnetic Susceptibility and Equilibrium Diagram of PdH<sub>n</sub>*, Berichte der Bunsengesellschaft für physikalische Chemie **77**, 48 (1973). doi:[10.1002/bbpc.19730770112](https://doi.org/10.1002/bbpc.19730770112).
- [2] R. Lässer and K. H. Klatt, *Solubility of hydrogen isotopes in palladium*, Physical Review B **28**, 748 (1983). doi:[10.1103/PhysRevB.28.748](https://doi.org/10.1103/PhysRevB.28.748).
- [3] C. Picard, O. J. Kleppa, and G. Boureau, *A thermodynamic study of the palladium–hydrogen system at 245–352°C and at pressures up to 34 atm*, The Journal of Chemical Physics **69**, 5549 (1978). doi:[10.1063/1.436550](https://doi.org/10.1063/1.436550).
- [4] R. Bardhan, L. O. Hedges, C. L. Pint, A. Javey, S. Whitlam, and J. J. Urban, *Uncovering the intrinsic size dependence of hydriding phase transformations in nanocrystals*, Nature Materials **12**, 905 (2013). doi:[10.1038/nmat3716](https://doi.org/10.1038/nmat3716).
- [5] T. B. Flanagan and D. Wang, *Low temperature hydrogen and deuterium isotherms for Pd and some of its binary alloys*, Journal of Alloys and Compounds , 157434 (2020). doi:[10.1016/j.jallcom.2020.157434](https://doi.org/10.1016/j.jallcom.2020.157434).
- [6] D. Foreman-Mackey, *corner.py: Scatterplot matrices in Python*, The Journal of Open Source Software **1**, 24 (2016). doi:[10.21105/joss.00024](https://doi.org/10.21105/joss.00024).
